# Supplementary material for: Public Signaling in Bayesian Ad Auctions
Source: arXiv:2201.09728 source file (2022-01-24)
Supplement: Supplementary file 1 [file appendix.tex]

\section{Appendice}
